# Supplementary material for: Multi-Agent Inverse Reinforcement Learning in Real World Unstructured Pedestrian Crowds
Source: arXiv:2405.16439 source file (2025-03-26)
Supplement: Supplementary file 1 [file appendix.tex]

\section{More Baselines and Results}
\label{sec: appendix}
We briefly discuss two important baselines that failed on the Speedway dataset.

\subsection{Hybrid IRL-BC}
Despite its simplicity and practical results in allowing robots to generalize complex behaviors to new and unstructured scenarios~\cite{xiao2022autonomous}, BC often suffers from compounding errors due to the fundamental design of the policy itself. In light of these challenges, Florence et al.~\cite{florence2022implicit} proposed a novel hybrid model that synergizes the principles of IRL and BC. This model is designed to uncover the underlying structures and ``rewards'' guiding expert behavior while preserving the practical and applicable nature of BC. This approach reformulates BC using implicit models, specifically, by employing the composition of $\arg\min$ with a continuous energy function $E_{\theta}$ to represent the policy $\pi_{\theta}$ as:

{\small\[
u^i_t = \arg\min_{\mathcal{U}^i} E_{\theta}(x_t, u^i_t)
\]}
This reformulation allows the representation of policies implicitly and formulates imitation as a conditional Energy-Based Modeling (EBM) problem, optimizing actions by minimizing a continuous energy function conditioned on the observations. 
% By integrating the inferred underlying structures of the expert’s behavior, akin to IRL, with the simplicity and direct applicability of BC, this model is considered as a hybrid IRL-BC approach. 
\begin{figure}[t]
\centering
   \begin{subfigure}[h]{0.485\columnwidth}
    \includegraphics[width=\textwidth]{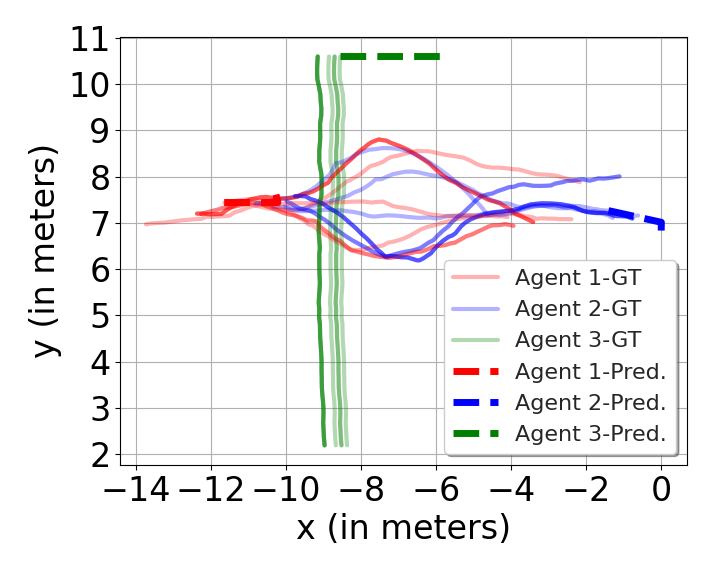}
    \caption{Implicit BC~\cite{florence2022implicit}}
    \label{fig: ibc}
  \end{subfigure}
  %
  %  \begin{subfigure}[h]{0.24\textwidth}
  %   \includegraphics[width=\textwidth]{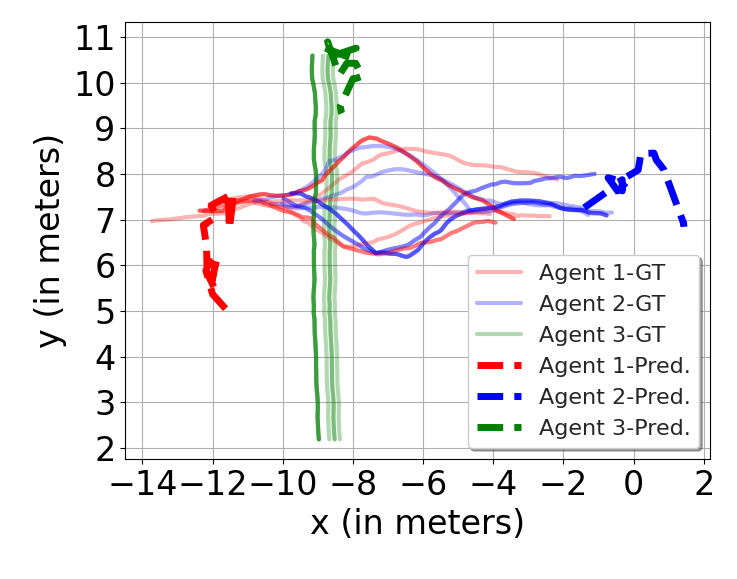}
  %   \caption{GMM-MLP}
  %   \label{fig: gmmmlp}
  % \end{subfigure}
  % %
  %  \begin{subfigure}[h]{0.24\textwidth}
  %   \includegraphics[width=\textwidth]{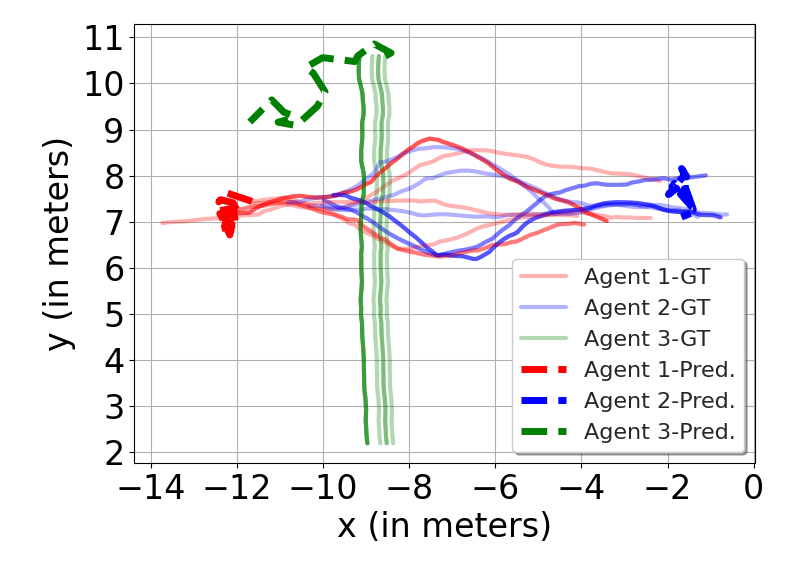}
  %   \caption{GMM-LSTM}
  %   \label{fig: gmmlstm}
  % \end{subfigure}
  %
     \begin{subfigure}[h]{0.485\columnwidth}
    \includegraphics[width=\textwidth]{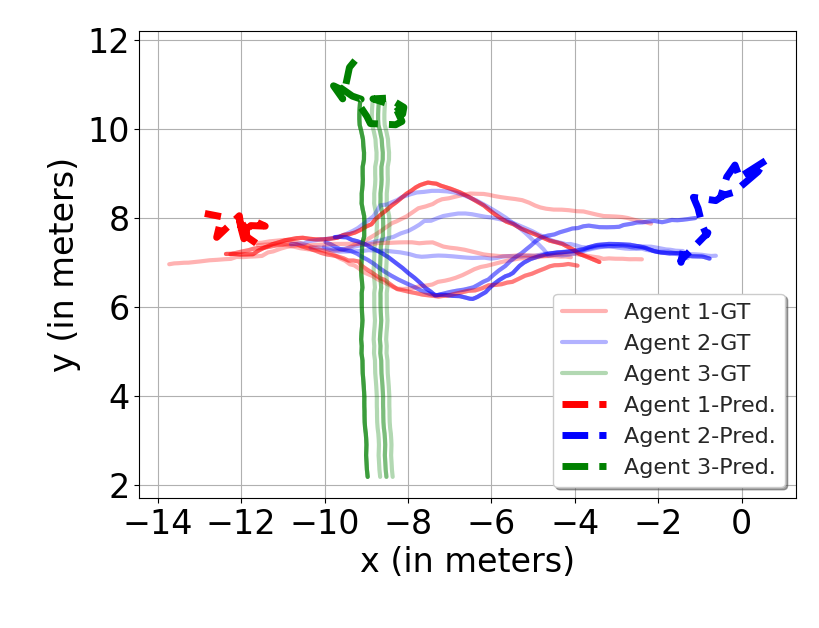}
    \caption{GMM}
    \label{fig: gmmtransformer}
  \end{subfigure}
\caption{Two additional baselines.} 
  \label{fig: main_results_2}
  \vspace{-10pt}
\end{figure}  

\subsection{Gaussian Mixture Models}
Here, we discuss Gaussian Mixture Models (GMMs) that estimate the parameters---means ($\mu$) and covariances ($\Sigma$)---of fixed Gaussian components. Each Gaussian component in the model represents a potential behavior for the agent, symbolizing unique sets of actions associated with specific states, and is characterized by the probability density function:

{\small\[ P(x) = \frac{1}{\sqrt{(2\pi)^k|\Sigma|}} \exp\left(-\frac{1}{2}(x_t-\mu)^T \Sigma^{-1} (x_t-\mu)\right) \]
}
% By learning the statistical properties embedded in these components, generative models are capable of producing actions and data points that are coherent with observed behaviors, thereby allowing for a comprehensive understanding and representation of the variability and diversity inherent in agent actions. 
Once the model has learned the parameters, it predicts actions by sampling from the established distributions using  $u^i_t \sim \mathcal{N}(\mu, \Sigma)$, where $u^i_t$ is the sampled action for $i$ at time $t$. The model comprises two hidden layers with $64$ units each and a dropout rate of $0.2$. We use the AdamW optimizer with Mean Squared Error (MSE) as the loss function. The learning rate is set to $3 \times 10^{-4}$, and mini-batch training is performed with a batch size of 64. A 60-40 cross-validation split is used for model assessment.

However, as shown in Figure~\ref{fig: main_results_2}, both the hybrid approach and GMMs failed to capture the multi-agent nature of IL.
% This process of learning and sampling provides insights into the plausible behaviors of agents, enabling the generation of actions that are not only consistent with observed data but also depict the dependencies and variations among different states and actions. In short, generative models serve as tools for capturing and simulating the many possible behaviors in agents by leveraging the relationships and distributions inherent in their actions and states.
